# Supplementary material for: Interpreting Rate-Distortion of Variational Autoencoder and Using Model Uncertainty for Anomaly Detection
Source: arXiv:2005.01889 source file (2020-05-07)
Supplement: Supplementary file 1 [file 8appendix.tex]

\section{More Experiment Results}
\input{8cifar10_table.tex}

\begin{figure*}[ht]
\vskip 0.2in
\begin{subfigure}[c]{0.333\textwidth}
\centering
\includegraphics[width=0.9\columnwidth]{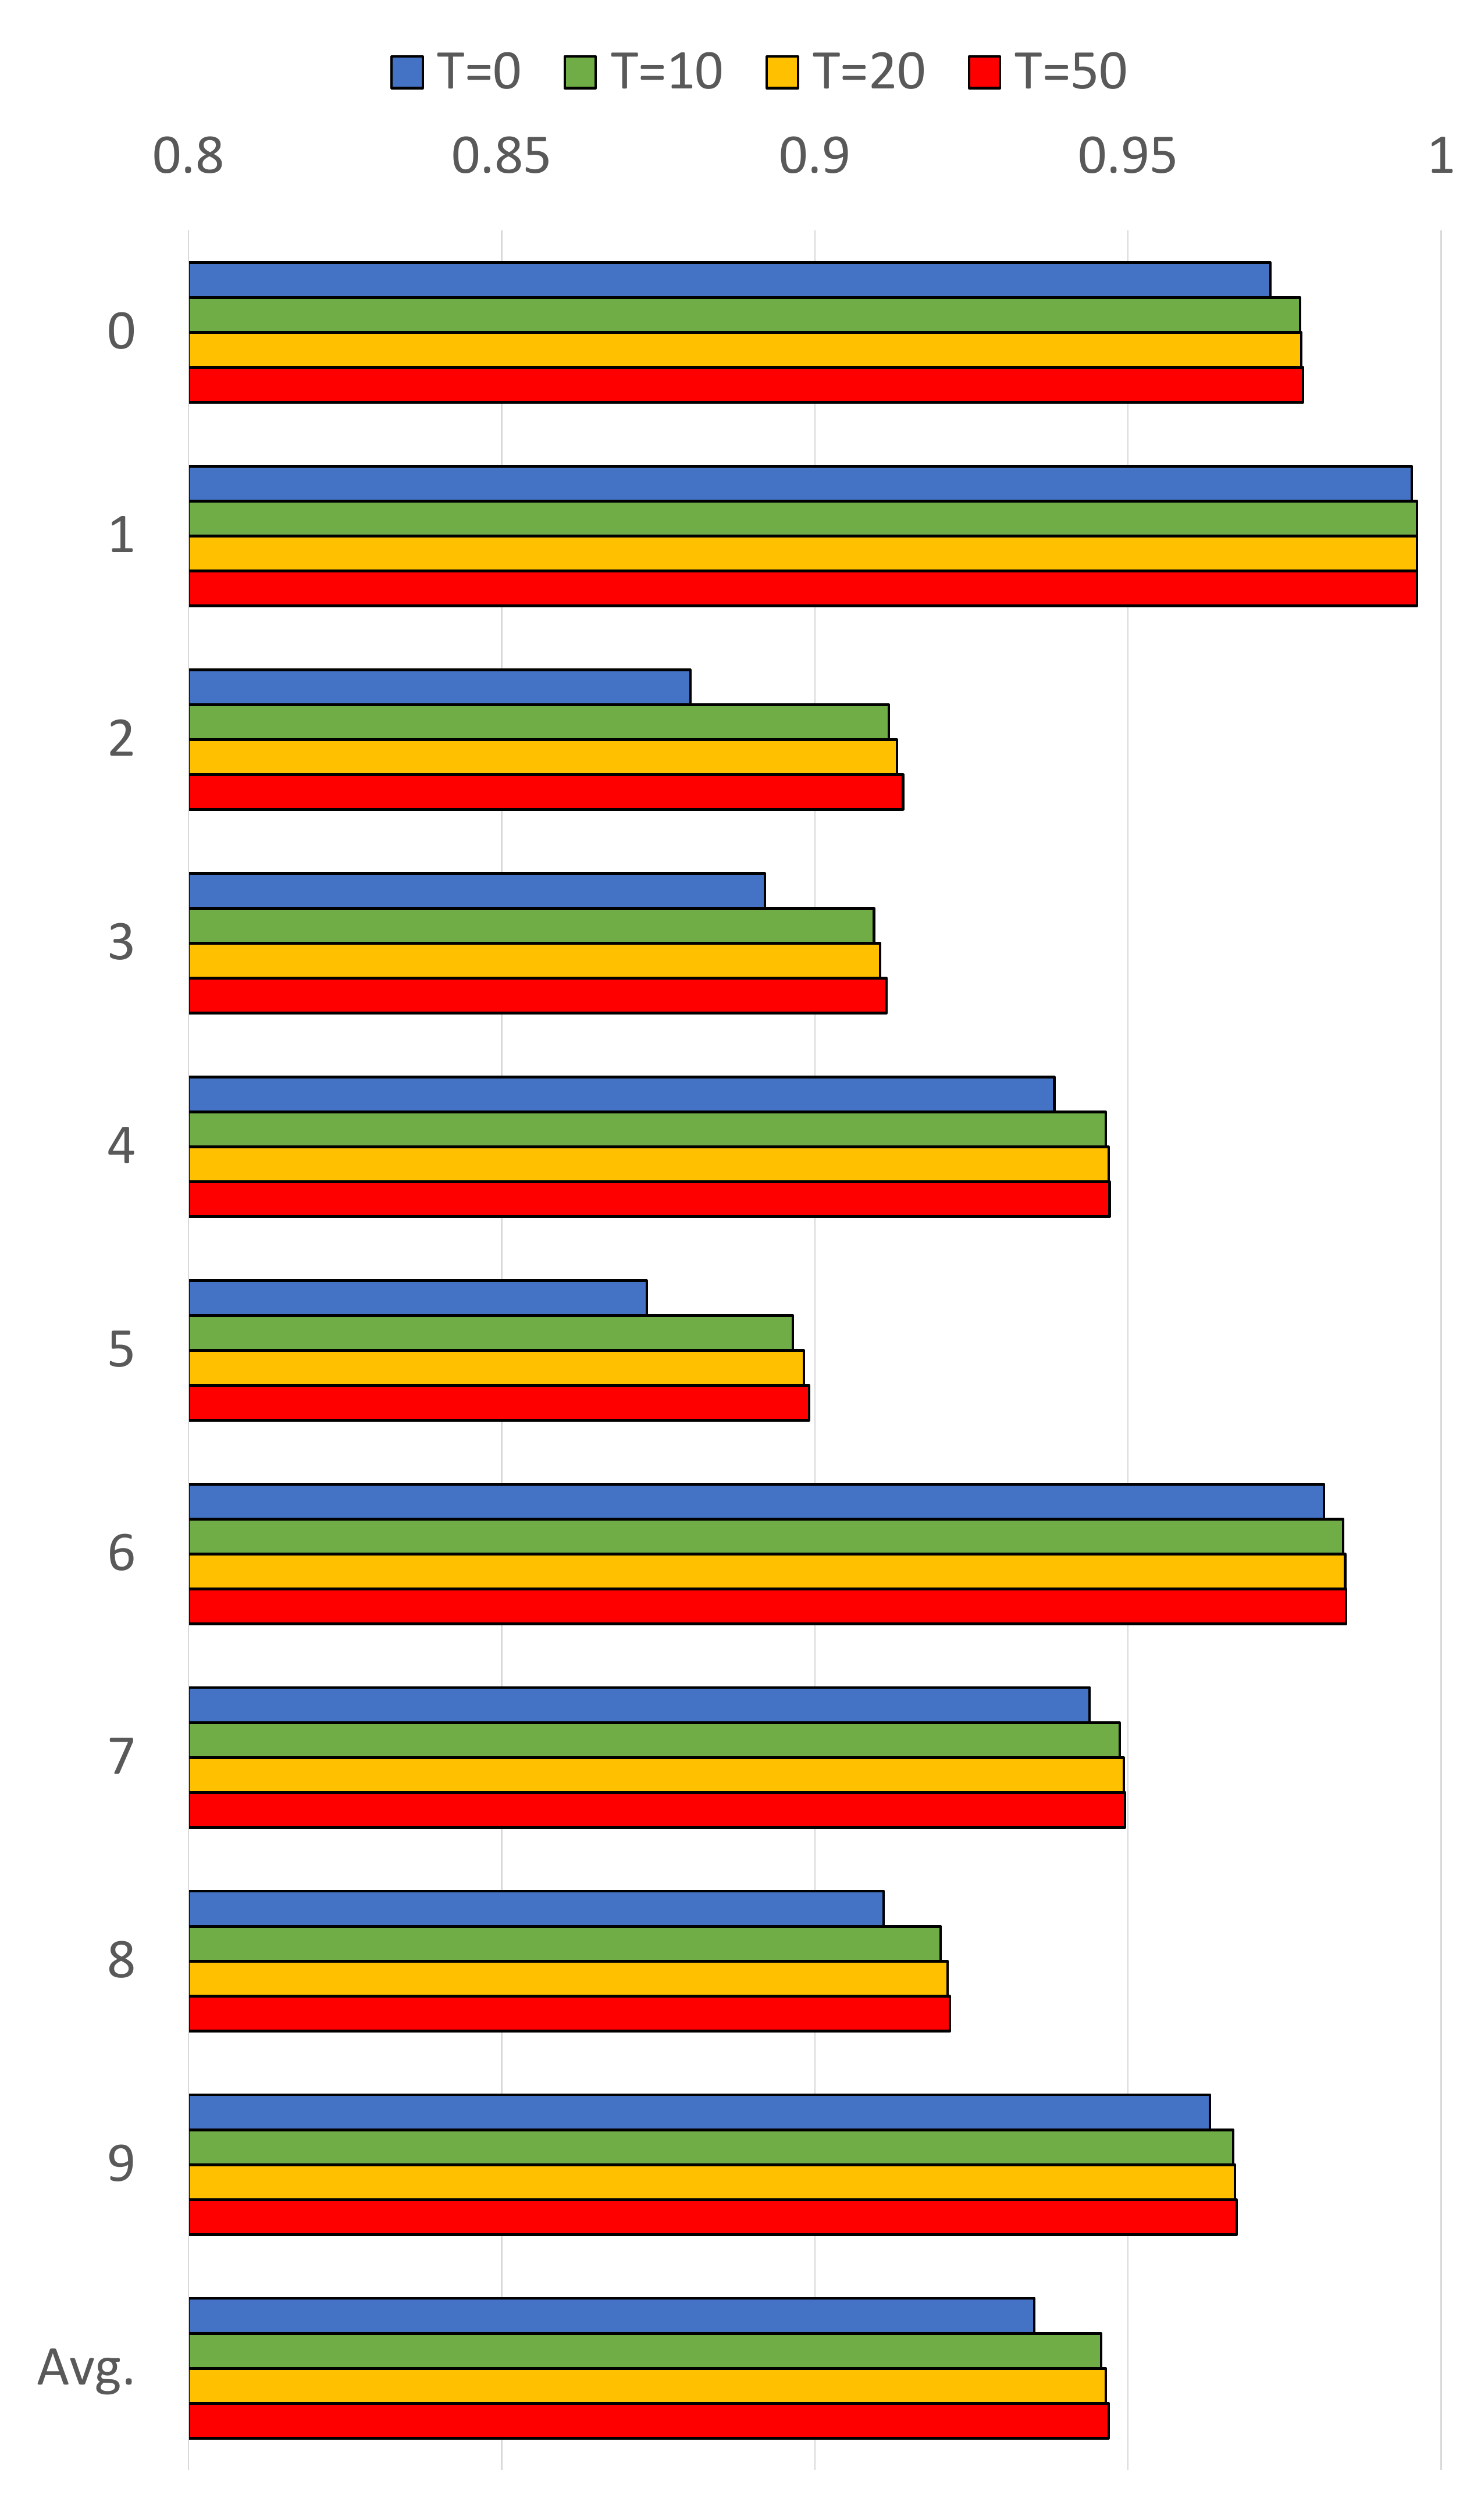}
\caption{MNIST}\label{subfig:mnist}
\end{subfigure}\hspace{-8mm}
\begin{subfigure}[c]{0.333\textwidth}
\centering
\includegraphics[width=0.9\columnwidth]{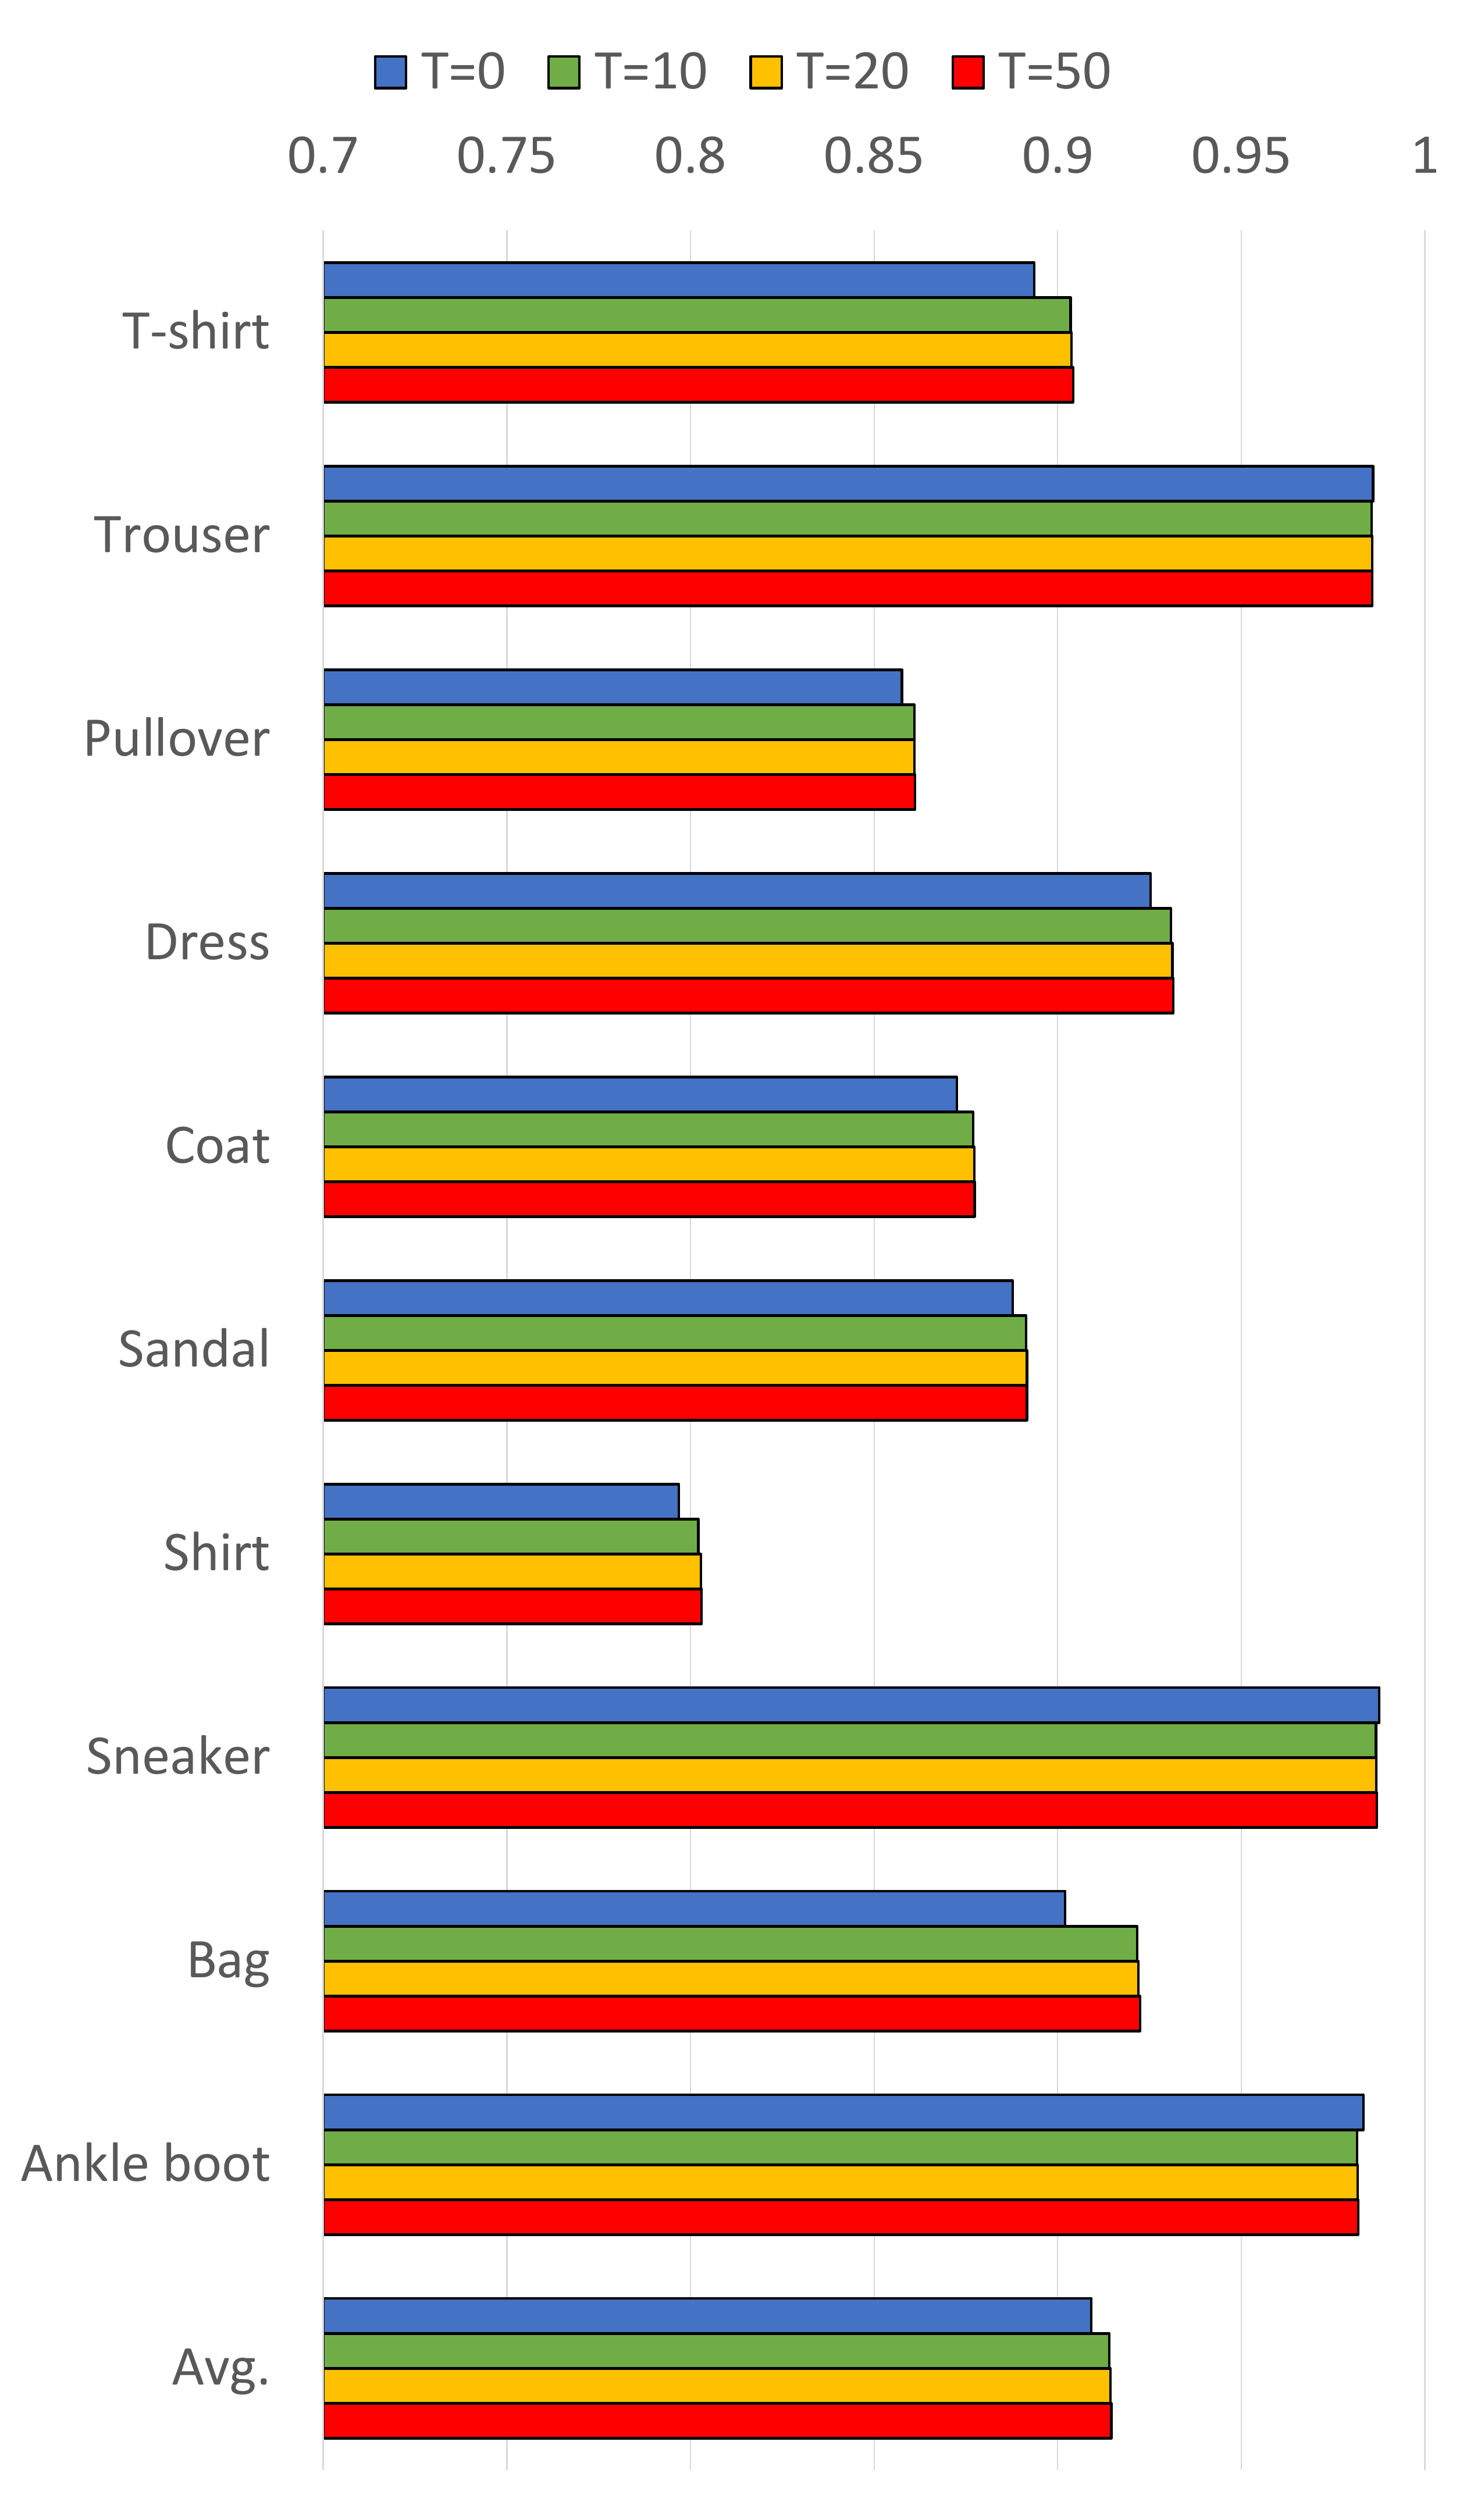}
\caption{FMNIST}\label{subfig:fmnist}
\end{subfigure}\hspace{-4mm}
\begin{subfigure}[c]{0.333\textwidth}
\centering
\includegraphics[width=0.9\columnwidth]{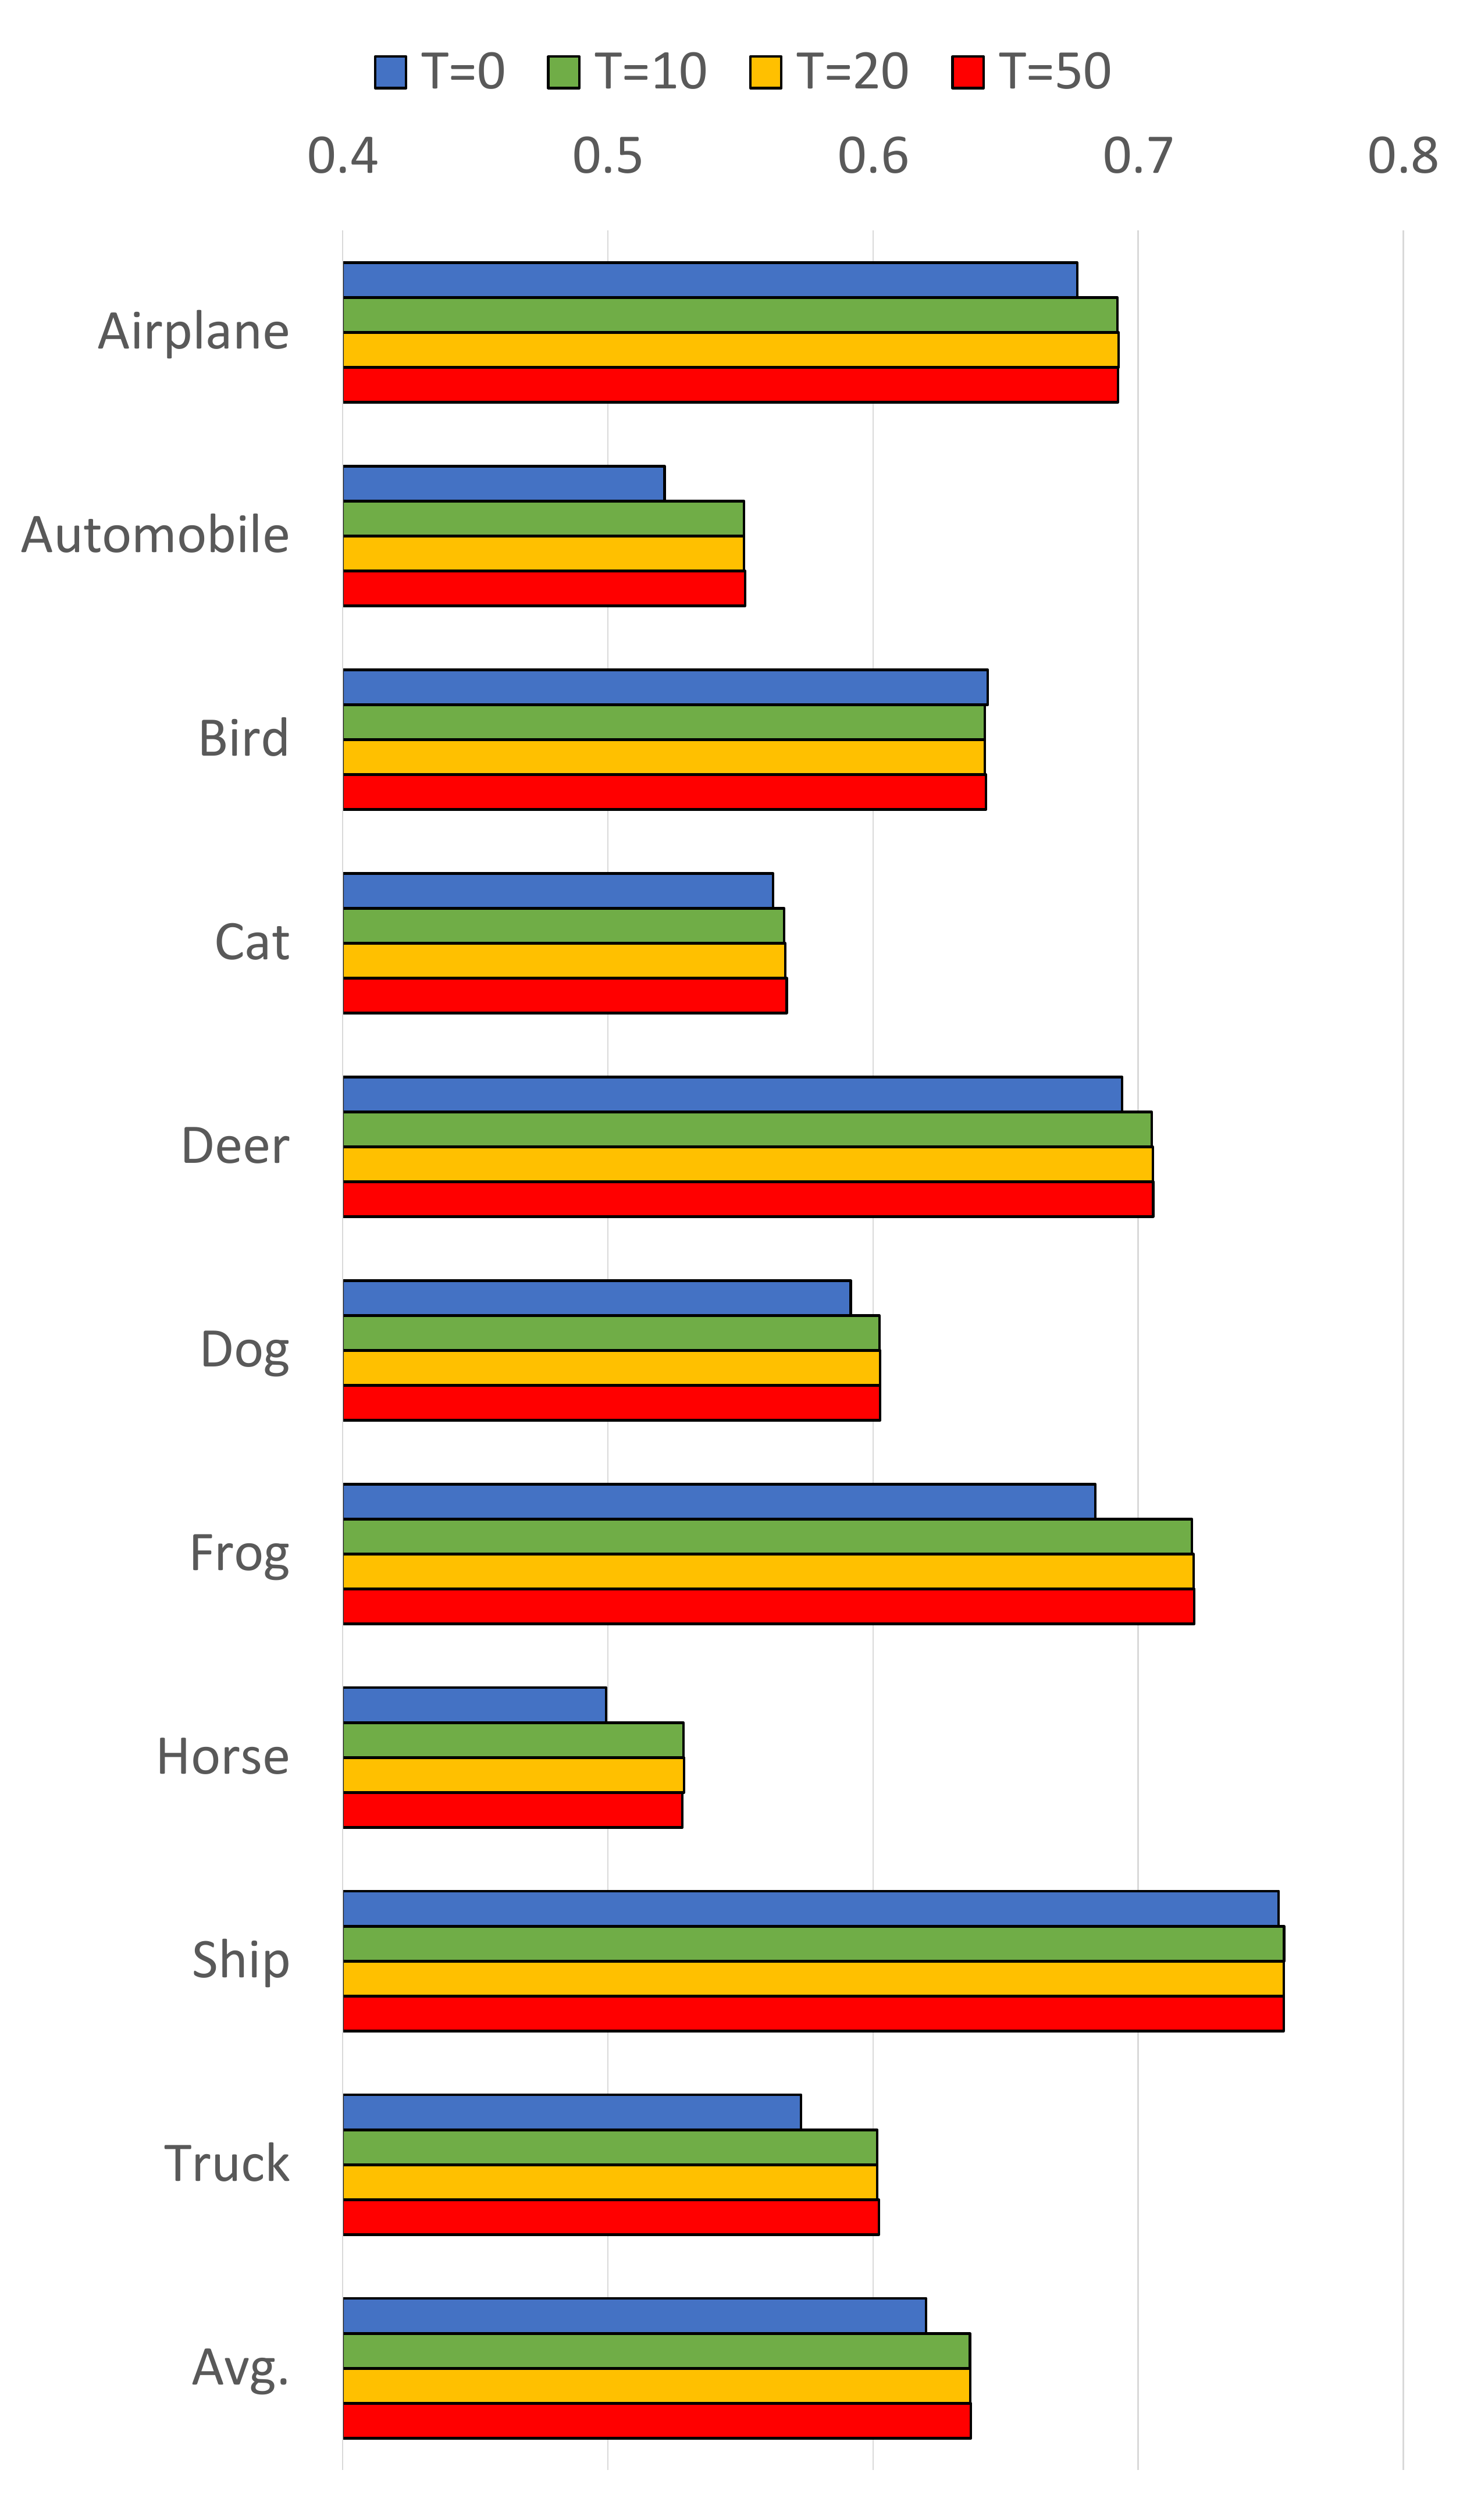}
\caption{CIFAR10}\label{subfig:cifar10}
\end{subfigure}
\vskip 0.2in
\caption{Ablation experiment results of model uncertainty metric of GPN on MNIST, FMNIST and CIFAR10 datasets. The values represent AUROCs [\%] with 10 different seeds.
}\label{fig:fig4}
\end{figure*}
